# Supplementary material for: Local Balance Calibration for Nonparametric Propensity Score Estimation
Source: arXiv:2404.04794 source file (2026-04-08)
Supplement: Supplementary file 1 [file KS1k_Ytable.tex]

\begin{table}[h]
\caption{The estimation of ATE by the four propensity score estimation methods in the \citet{kang2007demystifying} simulations with $N = 1,000$. The percent bias (Bias $\%$), root mean squared error (RMSE), empirical variance (VAR) are calculated from 100 Monte Carlo repetitions.}
\vskip 0.15in
\begin{center}
\begin{small}
\begin{sc}
\begin{tabular}{ccccccc}
\toprule
\multicolumn{1}{c}{ } & \multicolumn{3}{c}{Correctly Specified Model} & \multicolumn{3}{c}{Mis-specified Model} \\
\cmidrule(l{3pt}r{3pt}){2-4} \cmidrule(l{3pt}r{3pt}){5-7}
\multicolumn{1}{c}{Method} & \multicolumn{1}{c}{Bias\%} & \multicolumn{1}{c}{RMSE} & \multicolumn{1}{c}{Var} & \multicolumn{1}{c}{Bias\%} & \multicolumn{1}{c}{RMSE} & \multicolumn{1}{c}{Var} \\
\cmidrule(l{3pt}r{3pt}){1-1} \cmidrule(l{3pt}r{3pt}){2-2} \cmidrule(l{3pt}r{3pt}){3-3} \cmidrule(l{3pt}r{3pt}){4-4} \cmidrule(l{3pt}r{3pt}){5-5} \cmidrule(l{3pt}r{3pt}){6-6} \cmidrule(l{3pt}r{3pt}){7-7}
{True PS} & {0.1663} & {2.0688} & {4.2002} & {-} & {-} & {-}\\
Logistic & 0.0472 & 1.6536 & 2.7522 & 1.8127 & 8.6596 & 61.1095\\
{CBPS} & {0.0213} & {1.3535} & {1.8484} & {-0.6406} & {1.835} & {1.5732}\\
BCE & -0.0911 & 1.5733 & 2.4633 & -0.5305 & 2.0101 & 2.8277\\
{LBC-Net} & {-0.0723} & {1.1224} & {1.2493} & {-0.5255} & {1.6821} & {1.6277}\\
\bottomrule
\end{tabular}
\end{sc}
\end{small}
\end{center}
\vskip -0.1in
\label{tab:KS.Table1000}
\end{table}
