# Supplementary material for: Local Balance Calibration for Nonparametric Propensity Score Estimation
Source: arXiv:2404.04794 source file (2026-04-08)
Supplement: Supplementary file 2 [file SSMR_ATEtable.tex]

\begin{table}[h!]
\caption{The estimation of ATE by the four propensity score estimation methods in the SSMR simulations. The percent bias ($\%$bias), root mean squared error (RMSE), empirical variance (VAR) are calculated from $100$ Monte Carlo repetitions. The true ATE is $1$.}
\vskip 0.15in
\begin{center}
\begin{small}
\begin{sc}
\begin{tabular}{ccccccc}
\toprule
\multicolumn{1}{c}{ } & \multicolumn{3}{c}{Correctly Specified Model} & \multicolumn{3}{c}{Mis-specified Model} \\
\cmidrule(l{3pt}r{3pt}){2-4} \cmidrule(l{3pt}r{3pt}){5-7}
\multicolumn{1}{c}{Method} & \multicolumn{1}{c}{\%Bias} & \multicolumn{1}{c}{RMSE} & \multicolumn{1}{c}{Var} & \multicolumn{1}{c}{\%Bias} & \multicolumn{1}{c}{RMSE} & \multicolumn{1}{c}{Var} \\
\cmidrule(l{3pt}r{3pt}){1-1} \cmidrule(l{3pt}r{3pt}){2-2} \cmidrule(l{3pt}r{3pt}){3-3} \cmidrule(l{3pt}r{3pt}){4-4} \cmidrule(l{3pt}r{3pt}){5-5} \cmidrule(l{3pt}r{3pt}){6-6} \cmidrule(l{3pt}r{3pt}){7-7}
{Logistic} & {0.5497} & {0.0919} & {0.0085} & {-3.0341} & {0.1410} & {0.0192}\\
CBPS & -4.1804 & 0.0677 & 0.0029 & -6.2484 & 0.0932 & 0.0048\\
{BCE} & {3.8511} & {0.1617} & {0.0249} & {1.4358} & {0.2337} & {0.0550}\\
LBC-Net & 1.1318 & 0.0399 & 0.0015 & -0.6254 & 0.0304 & 0.0009\\
\bottomrule
\end{tabular}
\end{sc}
\end{small}
\end{center}
\vskip -0.1in
\label{tab:SSMR.ate}
\end{table}
